# Supplementary material for: Omni6DPose: A Benchmark and Model for Universal 6D Object Pose Estimation and Tracking
Source: arXiv:2406.04316 source file (2024-06-06)
Supplement: Supplementary file 1 [file 08_supp_abstract.tex]

This supplementary material provides additional statistics of {\Dataset}, visualization of {\SimData} dataset, the details of {\ModelName} implementation, and additional experiments and analysis.
